# Supplementary material for: Seeing the Image: Prioritizing Visual Correlation by Contrastive Alignment
Source: arXiv:2405.17871 source file (2024-11-05)
Supplement: Supplementary file 1 [file appendix_argen.tex]

% \begin{table}[t!]
%   \centering
%   \small
%   \renewcommand{\arraystretch}{1.2}
%   \caption{Detailed results of applying CAL to the LlamaGen~\cite{} Model}
%     \begin{tabular}{c|l|c|c|c|c|c}
%     \hline
%     Model & \#Para. & FID$\downarrow$ & IS$\uparrow$ & Precision$\uparrow$ & Recall$\uparrow$ \\ 
%     \hline
%     BigGAN~\cite{brock2018large} & 112M & 6.95 & 224.5 & 0.89 & 0.38 \\ \cline{1-6} 
%     GigaGAN~\cite{kang2023scaling} & 569M & 3.45 & 225.5 & 0.84 & 0.61 \\ \cline{2-7} 
%     StyleGAN-XL~\cite{sauer2022stylegan} & 166M & 2.30 & 265.1 & 0.78 & 0.53 \\ \hline
%     \end{tabular}
%   \label{tab:argen}
% \end{table}

\begin{table}[htbp]
\centering

\caption{Detailed Results of Applying Our Method to the LlamaGen~\cite{sun2024autoregressive} Model. Condition tokens are treated as the image token within the CAL method.}
\begin{tabular}{l|c|c|c|c|c|c|c}
\hline
Model & \#Parms & \textit{CAL} & Image-size & cfg & FID$\downarrow$ & rFID$\downarrow$ & IS$\uparrow$ \\ \hline
\multirow{4}{*}{GPT-B} & \multirow{4}{*}{111M} &     & 256 & 2.00 &      &      &      \\ \cline{3-8}
                       &                       & \checkmark & 256 & 2.00 &      &      &      \\ \cline{3-8}
                       &                       &     & 256 & 1.75 &      &      &      \\ \cline{3-8}
                       &                       & \checkmark & 256 & 1.75 &      &      &      \\ \hline
\multirow{4}{*}{GPT-XL} & \multirow{4}{*}{775M} &     & 256 & 1.75 & 3.17 & 7.16 & 272.19 \\ \cline{3-8}
                        &                       & \checkmark & 256 & 1.75 & 3.39 & 6.41 & 307.21 \\ \cline{3-8}
                        &                       &     & 256 & 1.50 & 3.14     &6.80      &228.37      \\ \cline{3-8}
                        &                       & \checkmark & 256 & 1.50 &2.80      &6.04      &256.31      \\ \hline
\end{tabular}
\label{tab:argen}
\end{table}
